# Supplementary material for: Bandit Learning with Delayed Impact of Actions
Source: arXiv:2002.10316 source file (2021-10-31)
Supplement: Supplementary file 1 [file appendix.tex]

% --------------------------------------------------------------
\section{Related Work} \label{related_work_full}
This work is related to several different areas: Lipschtiz bandit, combinatorial bandit, non-stationary bandit and long-term effect of decisions. 
Below we outline connections to each of these areas.

% --------------------------------------------------------------
\section{Missing Proofs for Action-Dependent Bandits} \label{proof_of_Action-Dependent_Bandits}

\subsection{Proof of Theorem \ref{theorem:regret_bound_naive}}
\begin{proof}
As mentioned, we \emph{uniformly discretize} the interval $[0, 1]$ of each arm into intervals of a fixed length $\epsilon$. 
Let $\{p_{k,1}, ..., p_{k,n}\}$ denote the \emph{discretized arms} for arm $k$, where $n = \left \lfloor 1/\epsilon  \right \rfloor$. 
% Note that $p_{k,j} = \epsilon(j-1)$.
Then the strategy space will be reduced as $\cP_\epsilon = \{p_{k,j}\}_{k\in[K], j\in [n]}$. 
We use this discretized strategy space $\cP_\epsilon$ as an approximation for the full set $\cP$.
Then the original infinite action space will be reduces as finite $\cP_\epsilon$, and we run an off-the-shelf MAB algorithm $\cA$, such as UCB1 or Successive Elimination, that only considers these actions in $\cP_\epsilon$. 
Adding more points to $\cP_\epsilon$ makes it a better approximation of $\cP$, but also increases regret of $\cA$ on $\cP_\epsilon$. 
Thus, $\cP_\epsilon$ should be chosen so as to optimize this tradeoff.

% One simple and natural solution is to \emph{uniformly discretize} the interval $[0,1]$ of each arm into a intervals of fixed length $\epsilon$, so that $\cP_\epsilon$ consists of all integer multiples of $\epsilon$ in $K$ dimensional.
We define $\Pi_\epsilon = \{\vp: \sum_{p_{k,j_k} \in \vp} p_{k,j_k }= 1, p_{k,j_k} \in \cP_\epsilon\} \subseteq \cP_{\epsilon}$, i.e., $|\Pi_\epsilon| = (\frac{1}{\epsilon} + 1)^{K-1}$.
Let the best strategy $\vp_\epsilon^* := \sup_{\vp \in \cP_\epsilon} \sum_{p_k \in \vp}p_k\mu_k(p_k)$. 
% which can be achived by solving following \emph{nonlinear} optimization problem:
% \begin{align*}
% \max_{\vp \in \cP_\epsilon} & \quad  \sum_{k \in [K]} p_k \mu_k(p_k) \\
% \text{s.t.}  	   & \quad  \sum_{k\in[K] } p_k= 1 \\
% 				   & \quad  p_k \geq 0 \quad \forall k
% \end{align*}
At each round, the algorithm $\cA$ can only hope to approach expected reward $U(\vp_\epsilon^*)$, and together with additionally suffering \emph{discretization error}:
\[
\DE_\epsilon = U(\vp^*) - U(\vp_\epsilon^*).
\]
Then the expected regret of the entire algorithm is:
\begin{align*}
\E[R(T)] & = T \cdot U(\vp^*) - \texttt{Reward}(\cA) \\
& = T \cdot U(\vp_\epsilon^*) - \texttt{Reward}(\cA) + T(U(\vp^*) - U(\vp_\epsilon^*)) \\
& = \E[R_{\epsilon} (T)]+ T \cdot \DE_\epsilon,
\end{align*}
where $\texttt{Reward}(\cA)$ is the total reward of the algorithm, and $R_{\epsilon} (T)$ is the regret relative to $U(\vp_\epsilon^*)$.
If $\cA$ attains optimal regret $\cO(\sqrt{NT \log T} )$ on any problem instance with time horizon $T$ and $N$ arms, then, 
\[
\E[R(T)] \leq \cO(\sqrt{\big|\Pi_{\epsilon}\big| T \log T} ) + T \cdot \DE_\epsilon.
\]
Thus, we need to choose $\epsilon$ to get the optimal trade-off between the size of $\cP_\epsilon$ and its discretization error.
Note that we could bound the $\DE_\epsilon$ by restricting $\vp_\epsilon^*$ to be nearest w.r.t $\vp^*$. 
Assume for each arm $k\in[K]$, we have following Lipschitz property:
\begin{align}
|\mu_k(p_1) - \mu_k(p_2)| \leq L_k|p_1-p_2|.
\end{align}
% Let $S = \sum_{k\in[K]} u_k$ and $u^* = \max_{k\in[K]} u_k$
Let $L^* = \max_{k\in[K]} L_k$, then it's easy to see that
\[
% \DE_\epsilon \leq \frac{L\epsilon}{2}(S + (K-2)u^*) \leq (K-1)L^*\epsilon
\DE_\epsilon = \Omega(KL^*\epsilon).
\]
Thus, the total regret can be bounded above from:
\[
\E[R(T)] \leq \cO\bigg(\sqrt{(1/\epsilon + 1)^{K-1} T \log T} \bigg) + \Omega(TKL^*\epsilon).
\]
By choosing $\epsilon = \big( \frac{\log T}{T(L^*)^2}\big)^{\frac{1}{K+1}}$ we obtain:
\[
\E[R(T)] \leq \cO(cT^{\frac{K}{K+1}}{(\log T)}^{\frac{1}{K+1}}).
\]
where $c = \Omega\big(K(L^*)^{\frac{K-1}{K+1}}\big)$.
\end{proof}

% ====================================

\subsection{Proof of Lemma \ref{lemma:key_lemma_vanilla}}\label{proof_of_lemma:key_lemma_vanilla}
\begin{proof}
By the defintion of the constructed $\UCB$, we then have:
\begin{align*}
\UCB_t(\vp) & = \sum_{k=1}^K p_{k, j_k}\bar{r}_t(p_{k, j_k}) + \sqrt{\ln t \frac{K}{n_t(\underline{p}_{k,j_k})}} \\
& \leq \sum_{k=1}^K p_{k, j_k}\bar{r}_t(p_{k, j_k}) + \frac{\Delta_{\vp}}{2}  \\
& < \big(\sum_{k=1}^K p_{k,j_k}\mu_k(p_{k,j_k}) + \frac{\Delta_{\vp}}{2}\big) + \frac{\Delta_{\vp}}{2} & \\
% \hspace{3em}& \rlap{\footnotesize by (\ref{useful_bound_2})} \\
& = \sum_{k=1}^K p_{k,j_k^*}\mu_k(p_{k,j_k^*}) < \sum_{k=1}^K p_{k,j_k^*}\bar{r}_t(p_{k,j_k^*}) + \sqrt{\ln t \frac{K}{n_t(\underline{p}_{k,j_k})}}  \\
% & \hspace{3em}& \rlap{\footnotesize by (\ref{useful_bound_1})}\\
& = \UCB_{t}(\vp^*),
\end{align*}
where $\underline{p}_{k,j_{k}}^* = \argmin_{p_{k,j_k}\in \vp^*} n_t(\underline{p}_{k,j_k})$.
The first inequality comes from that $n_t(\underline{p}_{k,j_k})\geq \frac{4K\ln t}{\Delta_{\vp}^2}$ and the probability of third inequality or fifth inequality not holding is at most $4/t^2$.
\end{proof}

% ====================================

\subsection{Proof of Lemma \ref{lemma: sufficient_sample}}\label{proof_of_lemma: sufficient_sample}
\begin{proof} 
For each suboptimal mixed strategy $\vp \neq \vp^*$, suppose there exists $\underline{p}_{k,j_k} \notin \vp^*$ such that $\underline{p}_{k,j_k} = \argmin_{p_{k,j_k} \in \vp} N_t(\cS(p_{k,j_k}))$. 
\begin{align*}
\Esymb[N_T(\cS(\underline{p}_{k,j_k}))] & = 1 + \Esymb \bigg[\sum_{t = n}^T \mathbbm{1}\big(\vp(t) = \vp, \vp\in \cS(\underline{p}_{k,j_k})\big)\bigg] \\
& = 1 + \Esymb \bigg[\sum_{t = n}^T \mathbbm{1}\big(\vp(t) = \vp, \vp\in \cS(\underline{p}_{k,j_k}); n_t(\underline{p}_{k,j_k}) < \frac{4K\ln t}{\Delta_{\vp}^2}\big)\bigg] \\
& \quad + \Esymb \bigg[\sum_{t = n}^T \mathbbm{1}\big(\vp(t) = \vp, \vp\in \cS(\underline{p}_{k,j_k}); n_t(\underline{p}_{k,j_k}) \geq \frac{4K\ln t}{\Delta_{\vp}^2}\big)\bigg] \\
& \leq \frac{4K\ln T}{\Delta_{\vp}^2} +  \Esymb \bigg[\sum_{t = n}^T \mathbbm{1}\big(\vp(t) = \vp, \vp\in \cS(\underline{p}_{k,j_k}); n_t(\underline{p}_{k,j_k}) \geq \frac{4K\ln t}{\Delta_{\vp}^2}\big)\bigg] \\
& = \frac{4K\ln T}{\Delta_{\vp}^2} +  \sum_{t = n}^T\Psymb \bigg(\vp(t) = \vp, \vp\in \cS(\underline{p}_{k,j_k}); n_t(\underline{p}_{k,j_k}) \geq \frac{4K\ln t}{\Delta_{\vp}^2}\bigg) \\
& = \frac{4K\ln T}{\Delta_{\vp}^2} +  \sum_{t = n}^T\Psymb \bigg(\vp(t) = \vp, \vp\in \cS(\underline{p}_{k,j_k})\bigg| n_t(\underline{p}_{k,j_k}) \geq \frac{4K\ln t}{\Delta_{\vp}^2} \bigg)\Psymb \bigg(n_t(\underline{p}_{k,j_k}) \geq \frac{4K\ln t}{\Delta_{\vp}^2}\bigg)\\
% & \leq  \frac{4K\ln T}{\Delta_{\vp}^2} + \sum_{t=n}^T \frac{4}{t^2}\\
& \leq \frac{4K\ln T}{\Delta_{\vp}^2} + \frac{2\pi^2}{3}.
\end{align*}
1 was added in the first equality to acconut for 1 initial pull of every meta arm by the algorithm.
For the first inequality, suppoese for contradiction that the indicator $\mathbbm{1}\big(\vp(t) = \vp, \vp\in \cS(\underline{p}_{k,j_k}); n_t(\underline{p}_{k,j_k}) < L\big)$ takes value of 1 at more than $L-1$ time steps, where $L = \frac{4K\ln T}{\Delta_{\vp}^2}$. 
Let $\tau$ be the time step at which this indicator is 1 for the $(L-1)-$th time.
Then the number of pulls of all meta arms in $\cS(\underline{p}_{k,j_k})$ is at least $L$ times until time $\tau$ (including the initial pull), and for all $t > \tau$, $n_t(\underline{p}_{k,j_k}) \geq L$ which implies $n_t(\underline{p}_{k,j_k}) \geq \frac{4K\ln t}{\Delta_{\vp}^2}$.
Thus, the indicator cannot be 1 for any $t\geq \tau$, contradicting the assumption that the indicator takes value of 1 more than $L$ times.
This bounds $1 + \Esymb \big[\sum_{t = n}^T \mathbbm{1}\big(\vp(t) = \vp, \vp\in \cS(\underline{p}_{k,j_k}); n_t(\underline{p}_{k,j_k}) < L\big)\big]$ by $L$.

For the second inequality, we apply the lemma \ref{lemma:key_lemma_vanilla} to bound the first conditional probability term and use the fact that the probabilities cannot exceed 1 to bound the second probability term.
\end{proof}

\subsection{Proof of Theorem \ref{theorem:key_theorem_vanilla}} \label{proof_of_theorem:key_theorem_vanilla}
Before proceeding to bound the regret, we define following statistics. 
Let $L^{p_{k,j_k}} = |\cS(p_{k,j_k})|$ denote the cardinality of the super set $\cS(p_{k,j_k})$.
We sort all the meta arms in $\cS(p_{k,j_k})$ as $\vp_1(p_{k,j_k}), ..., \vp_{L_{p_{k,j_k}}}(p_{k,j_k})$ in the order of increasing expected rewards.
Let $\Delta_l^{p_{k,j_k}} \overset{\Delta}{=} \Delta_{\vp_l(p_{k,j_k})}, \forall l\in [L_{p_{k,j_k}}]$.

Observe that according to lemma \ref{lemma: sufficient_sample}, at each round $t$, for each discretized arm $p_{k,j_k} \notin \vp^*$, there're two cases:
\squishlist
	\item There exists a meta arm $\vp$ such that $\vp \in \cS(p_{k,j_k})$, and $p_{k,j_k} = \argmin_{p_{k,j_k}\in\vp} N_t(\cS(p_{k,j_k}))$. 
	Then we can bound the total number of pulls for all $\vp \in \cS(p_{k,j_k})$ by $N_t(\cS(p_{k,j_k}))$, i.e.,
	\begin{align*}
	\sum_{\vp \in \cS(p_{k,j_k})} N_t(\vp) \leq N_t(\cS(p_{k,j_k})) \leq \frac{4K\ln t}{(\Delta_{\text{min}}^{p_{k,j_k}})^2} + \frac{2\pi^2}{3}.
	\end{align*}
	\item There exists no meta arm $\vp$ such that $\vp \in \cS(p_{k,j_k})$, and $p_{k,j_k} = \argmin_{p_{k,j_k}\in\vp} N_t(\cS(p_{k,j_k}))$. 
	In this case, for each $\vp_l \in \cS(p_{k,j_k})$, we can always find that there exists another discretized arm $p_l\in \vp_l(p_{k,j_k})$ but $p_l \neq p_{k,j_k}$ such that $p_l = \argmin_{p_{k,j_k}\in \vp_l(p_{k,j_k})} N_t(\cS(p_{k,j_k}))$.
	Thus, for each $\vp_l(p_{k,j_k}) \in \cS(p_{k,j_k})$, together with other meta arms which have the same discretized arm $p_l$ as $\vp_l(p_{k,j_k})$, i.e.,
	\begin{align*}
	\sum_{\vp \in \bigcup_{p_{l} \in \vp} \vp} N_t(\vp)  = \sum_{\vp\in \cS(p_l)}  N_t(\vp) = N_t(\cS(p_l)) \leq  
	\frac{4K\ln t}{(\Delta_{\text{min}}^{p_{l}})^2} + \frac{2\pi^2}{3}.
	\end{align*}
\squishend
% there exists $p_{\text{min}} \in \bigcup_{l=1}^{L^{p_{k,j_k}}} \vp_l(p_{k,j_k})$ such that 
% we have $\sum_{l\in [L^{p_k,j_k}]} N_t(\vp_l(p_{k,j_k}))\leq N_t(\underline{\cS})$, where $N_t(\underline{\cS}) \overset{\Delta}{=} \min_{p_{k,j_k}} N_t(\cS(p_{k,j_k}))$

Thus, for each discretized arm $p_{k,j_k}$, we can focus on the case where $p_{k,j_k}$ can attain the minimum $N_t(\cS(p_{k,j_k}))$ for  some $\vp \in \cS(p_{k,j_k})$.

Note that even though we can not find a meta arm $\vp \in \cS(p_{k,j_k})$ such that $p_{k,j_k} = \argmin_{p_{k,j_k}\in \vp} N_t(\cS(p_{k,j_k}))$, we can always apply similar analysis by finding another discretized arm $p_l \in \vp $ but $p_l \neq p_{k,j_k}$ such that $p_l = \argmin_{p_{k,j_k}\in \vp} N_t(\cS(p_{k,j_k}))$.

For each discretized arm $p_{k,j_k} \notin \vp^*$, define following property of its corresponding super arm: 
\begin{align*}
\Delta^{p_{k,j_k}}_{\text{min}} & := \min_{\vp\in \cS(p_{k,j_k})} \Delta_{\vp} = \Delta_{L_{p_{k,j_k}}}^{p_{k,j_k}}\\
\Delta^{p_{k,j_k}}_{\text{max}} & := \max_{\vp\in \cS(p_{k,j_k})} \Delta_{\vp} = \Delta_{1}^{p_{k,j_k}}.
\end{align*}
% We also define:
% \begin{align*}
% \Delta{\text{min}} & = \min_{p_{k,j_k}} \Delta^{p_{k,j_k}}_{\text{min}} \\
% \Delta{\text{max}} & = \max_{p_{k,j_k}} \Delta^{p_{k,j_k}}_{\text{max}}.
% \end{align*}
\ignore{

	One way is to rewrite the total regret as the following:
	\begin{align}
	\Esymb[R(t)] & = \sum_{\vp \neq \vp^*} N_t(\vp) \Delta_{\vp}\\
	& \leq \Delta_{\text{max}} \sum_{\vp \neq \vp^*} N_t(\vp)\\
	& \leq \Delta_{\text{max}} \sum_{p_{k,j_k} \notin \vp^*}\max_{\vp \in \cS(p_{k,j_k})}{}N_t(\cS(p_{k,j_k}))\\
	& \leq \Delta_{\text{max}} \sum_{p_{k,j_k} \notin \vp^*} \bigg(\frac{4K\ln t}{(\Delta_{\text{min}}^{p_{k,j_k}})^2} + \frac{2\pi^2}{3}\bigg)\\
	& \leq \Delta_{\text{max}}K\bigg(\frac{1}{\epsilon}-1\bigg)  \bigg(\frac{4K\ln t}{\Delta_{\text{min}}^2} + \frac{2\pi^2}{3}\bigg) \label{regret_1}
	\end{align}
	$\textbf{Optimizing Regret}$ (\ref{regret_1}). It's easy to see that $\Delta_{\text{min}} \geq \epsilon \cdot\min_{k} L_k$.
	Let $L_{\text{min}} =  \min_{k}L_k$.
	Combining the discretization error $\DE_\epsilon$, we have following:
	\begin{align}
	\Esymb[R(T)] \leq \frac{4(1-\epsilon)\Delta_{\text{max}} K^2\ln T }{\epsilon^3 L_{\text{min}}^2} + \frac{\Delta_{\text{max}}(1-\epsilon) KC_1}{\epsilon} + C_2T(K-1)\epsilon
	\end{align}
	Optimizing w.r.t $\epsilon$, i.e., let $\epsilon = \Theta\bigg(\big(\frac{K^2\ln T}{T(K-1)}\big)^{1/4}\bigg)$, we have:
	\begin{align}
	\Esymb[R(T)] \leq \cO(K^{5/4}T^{3/4}(\ln T)^{1/4})
	\end{align}
}
We now ready to warp up the proof of the total regret bound.
\begin{proof}
Observe that for each discretized arm not in the optimal arms, we can reduce the total regret into the following regret on pulling the meta arm which contains this \emph{suboptimal} discretized arm, i.e., 
\begin{align}
\Esymb[R(t)] & = \sum_{\vp \neq \vp^*} N_t(\vp) \Delta_{\vp}\\
& \leq \sum_{p_{k,j_k} \notin \vp^*} \sum_{l\in [L^{p_k,j_k}]} N_t(\vp_l(p_{k,j_k})) \Delta_l^{p_k,j_k}. \label{regret_2}
\end{align}

% \wt{need to add the proof on boudning the regret for sufficient samples for suboptimal meta arms}. 
\ignore{

	Observe that we can bound the $\sum_{l\in [L^{p_k,j_k}]} N_t(\vp_l(p_{k,j_k})) \Delta_l^{p_k,j_k}$ as the following:
	\begin{align}
	\sum_{l\in [L^{p_k,j_k}]} N_t(\vp_l(p_{k,j_k})) \Delta_l^{p_k,j_k} & = \sum_{l\in [L^{p_k,j_k}]} N_t(\vp_l(p_{k,j_k})) \Delta_{\text{min}}^{p_k,j_k} + N_t(\vp_l(p_{k,j_k})) (\Delta_l^{p_k,j_k} - \Delta_{\text{min}}^{p_k,j_k}) \\
	& = \Delta_{\text{min}}^{p_k,j_k}\sum_{l\in [L^{p_k,j_k}]}N_t(\vp_l(p_{k,j_k}))+ \sum_{l\in [L^{p_k,j_k}]}N_t(\vp_l(p_{k,j_k})) (\Delta_l^{p_k,j_k} - \Delta_{\text{min}}^{p_k,j_k}) \\
	& \leq \Delta_{\text{min}}^{p_k,j_k} \frac{4K\ln t}{\big(\Delta_{\text{min}}^{p_k,j_k}\big)^2} + \sum_{l\in [L^{p_k,j_k}]}N_t(\vp_l(p_{k,j_k})) (\Delta_l^{p_k,j_k} - \Delta_{\text{min}}^{p_k,j_k})
	\end{align}
}
\ignore{
	Then we can easily bound the total number of pulls of all suboptimal meta arms:
	\begin{align}
	\sum_{\vp \neq \vp^*} N_t(\vp) & 
	% \leq \sum_{\cS \in \Xi_\epsilon \setminus  \Xi_\epsilon(\vp^*)} N_t(\underline{\cS}) \\
	\leq \sum_{p_{k,j_k} \notin \vp^*} \frac{4K\ln t}{(\Delta^{p_{k,j_k}}_{\text{min}})^2} + C\\
	\text{or} & \leq K\big(\frac{1}{\epsilon}-1\big)  \big(\frac{4K\ln t}{\Delta_{\text{min}}^2} + C\big)
	\end{align}
}
Define $l_t(\Delta) \overset{\Delta}{=} \frac{4K\ln t}{\Delta^2} + \frac{2\pi^2}{3}$. 
Thus, for discretized arm $p_{k,j_k}$, its counter $N_t(\cS(p_{k,j_k}))$ will increase from 0 to $l_t(\Delta_\text{min}^{p{k,j_k}})$.
Suppoes from round $s-1$ to $s$ and assume $N_{s-1}(\cS(p_{k,j_k}))$ is in the range of $(l_t(\Delta_{j-1}^{p_{k,j_k}}), l_t(\Delta_j^{p_{k,j_k}})]$ for some $j \in [L^{p_{k,j_k}}]$, 
and on pulling the meta arm $\vp_l(p_{k,j_k})\in \cS(p_{k,j_k})$,  $N_s(\cS(p_{k,j_k}))$ increments 1, then we must have following:
% \begin{subequations}
\begin{align} 
\Delta_{l}^{p_{k,j_k}} & < \Delta_{j-1}^{p_{k,j_k}}  \label{ineq: relax_badness_1} \\
& \leq \Delta_{j}^{p_{k,j_k}}, \label{ineq: relax_badness_2} 
\end{align}
% \end{subequations}
where (\ref{ineq: relax_badness_1}) comes from lemma \ref{lemma: sufficient_sample}, since any suboptimal meta arms cannot be pulled with more than $l_t(\Delta_l^{p_{k,j_k}})$ times.
And (\ref{ineq: relax_badness_2}) comes from the defintion on $\Delta_l^{p_{k,j_k}}$.
Then we have following relaxation for the incurred regret:
\begin{align} \label{logics_end: relax gap}
\big(l_t(\Delta_j^{p_{k,j_k}}) - l_t(\Delta_{j-1}^{p_{k,j_k}})\big)\Delta_l^{p_{k,j_k}} \leq \big(l_t(\Delta_j^{p_{k,j_k}}) - l_t(\Delta_{j-1}^{p_{k,j_k}})\big)\Delta_j^{p_{k,j_k}}.
\end{align}
Thus, we can decompose the $\sum_{l\in [L^{p_k,j_k}]} N_t(\vp_l(p_{k,j_k})) \Delta_l^{p_k,j_k}$ as the following:
\begin{align*}
\sum_{l\in [L^{p_k,j_k}]} N_t(\vp_l(p_{k,j_k})) \Delta_l^{p_k,j_k} & \leq \sum_{j=1}^{L^{p_{k,j_k}}} \big(l_t(\Delta_j^{p_{k,j_k}}) - l_t(\Delta_{j-1}^{p_{k,j_k}})\big) \Delta_j^{p_{k,j_k}} \\
& = l_t(\Delta_\text{min}^{p_{k,j_k}})\Delta_\text{min}^{p_{k,j_k}} + \sum_{j \in [L^{p_{k,j_k}} - 1]}l_t(\Delta_j^{p_{k,j_k}})\cdot(\Delta_j^{p_{k,j_k}} - \Delta_{j+1}^{p_{k,j_k}}) \\
& \leq l_t(\Delta_\text{min}^{p_{k,j_k}})\Delta_\text{min}^{p_{k,j_k}} + \int_{\Delta_\text{min}^{p_{k,j_k}}}^{\Delta_\text{max}^{p_{k,j_k}}}l_t(x)dx \\
% & = \frac{4K\ln t}{(\Delta_\text{min}^{p_{k,j_k}})^2}\Delta_\text{min}^{p_{k,j_k}} + \int_{\Delta_\text{min}^{p_{k,j_k}}}^{\Delta_\text{max}^{p_{k,j_k}}}\frac{4K\ln t}{x^2}dx \\
& = \frac{4K\ln t}{\Delta_\text{min}^{p_{k,j_k}}}  + 4K\ln t \bigg(\frac{1}{\Delta_\text{min}^{p_{k,j_k}}} - \frac{1}{\Delta_\text{max}^{p_{k,j_k}}} \bigg) + \frac{2\pi^2}{3}\Delta_\text{max}^{p_{k,j_k}}
\end{align*}
Thus, regret (\ref{regret_2}) is equivalent to following \emph{instance-dependent} regret bound:
\begin{align*}
(\ref{regret_2}) \leq \sum_{p_{k,j_k} \notin \vp^*} \bigg(\frac{8K\ln t}{\Delta_\text{min}^{p_{k,j_k}}} - 4K\ln t + \frac{2\pi^2}{3}\Delta_\text{max}^{p_{k,j_k}}\bigg).
\end{align*}
To achieve \emph{instance-independent} regret bound, divide the super set (or the discretized arms) into two groups: 
% \wt{need more carefull to tune the thresholds}
% \squishlist
% 	\item Group 1 contains the super sets (or the discretized arms) which satisfy $\Delta^{p_{k,j_k}}_{\text{min}} \geq \sqrt{\frac{K}{\epsilon}\frac{\ln T}{T}}$;
% 	\item Group 2 contains the super sets (or the discretized arms) which satisfy $\Delta^{p_{k,j_k}}_{\text{min}} \leq \sqrt{\frac{K}{\epsilon}\frac{\ln T}{T}}$;
% \squishend
\squishlist
	\item Group 1 contains the super sets (or the discretized arms) which satisfy $\Delta^{p_{k,j_k}}_{\text{min}} \geq \sqrt{\frac{K^2\ln T}{\epsilon T}}$;
	\item Group 2 contains the super sets (or the discretized arms) which satisfy $\Delta^{p_{k,j_k}}_{\text{min}} \leq \sqrt{\frac{K^2\ln T}{\epsilon T}}$;
\squishend
Then the total regret is the sum of the regret of each group.
For the case 1, the maximum total regret incurred due to pulling the meta arms which are contained in the super set of the Group 1 is bounded by:
\begin{align*}
\sum_{\vp \in \{\bigcup_{\cS: \cS \in \text{Group 1}} \cS\}} N_T(\vp) \Delta_{\vp} & \leq \sum_{p_{k,j_k} \in \text{Group 1}} \bigg(\frac{8K\ln T}{\Delta_\text{min}^{p_{k,j_k}}} - 4K\ln T + \frac{2\pi^2}{3}\Delta_\text{max}^{p_{k,j_k}}\bigg) \\
& \leq \sum_{p_{k,j_k} \in \text{Group 1}} \bigg(\frac{8K\ln T}{\sqrt{\frac{K^2\ln T}{\epsilon T}}} - 4K\ln T + \frac{2\pi^2}{3}\Delta_\text{max}^{p_{k,j_k}}\bigg)\\
& \leq \frac{K}{\epsilon}\bigg(\frac{8K\ln T}{\sqrt{\frac{K^2\ln T}{\epsilon T}}}  - 4K\ln T +  \frac{2\pi^2}{3}\Delta_\text{max}^{p_{k,j_k}}\bigg)\\
& \leq 8K\sqrt{\frac{T\ln T}{\epsilon}} + \frac{2\pi^2K}{3\epsilon}- \frac{4K^2\ln T}{\epsilon}.
\end{align*}
Furthermore, the maximum total regret incurred due to pulling the meta arms which are contained in the super set of the Group 2 is bounded by:
\begin{align*}
\sum_{\vp \in \{\bigcup_{\cS: \cS \in \text{Group 2}} \cS\}} N_T(\vp) \Delta_{\vp} & \leq \sqrt{\frac{K^2\ln T}{\epsilon T}} \sum_{\vp \in \{\bigcup_{\cS: \cS \in \text{Group 2}} \cS\}} N_T(\vp)\leq \sqrt{\frac{T\ln T}{\epsilon}}.
\end{align*}
Combining the incurred regret on above two groups, the \emph{instance-independent} regert bound will be given as follows:
\begin{align*}
\Esymb_{\cA}[R(T)] \leq \cO\bigg(K\sqrt{\frac{T\ln T}{\epsilon}}\bigg).
\end{align*}
Together with the discretization error, we have,
\begin{align*}
\Esymb[R(T)] & \leq \cO\bigg(K\sqrt{\frac{T\ln T}{\epsilon}}\bigg) + \DE_\epsilon\\
& = \cO\bigg(K\sqrt{\frac{T\ln T}{\epsilon}}\bigg) + CT(K-1)\epsilon,
\end{align*}
and optimizing w.r.t $\epsilon$, i.e., $\epsilon = \Theta \bigg( T^{-1/3} (\ln T)^{1/3} \bigg)$.
We could obtain following total regret bound:
\begin{align*} \label{u_regret_bound:vanilla}
\Esymb[R(T)] \leq \cO(KT^{2/3}(\ln T)^{1/3}).
\end{align*}
\end{proof}

% --------------------------------------------------------------
\section{Missing Proofs for History-dependent Bandits}
\label{appendix: proofs_history_dependent_bandit}

\subsection{Proof of Lemma \ref{lemma: approx_err_neq_1}}\label{proof_lemma_approx_err_neq_1}
\begin{proof}
For analysis simplicity, let us suppose $t = mL$. 
For the ease of presentation, also let $t^\est_m \overset{\Delta}{=} \frac{t}{L}(L-s_a) = m(L-s_a)$ be the total number of estimation rounds in the first $m$ phases .
Thus, at the end of the approaching stage, we have
\begin{align*}
\hat{p}_{k, t+s_a}^\gamma = \frac{\mathbbm{1}_{(a_{t+s_a} = k|p_k)}\gamma^{0} + ...+\mathbbm{1}_{(a_{t+1} = k|p_k)}\gamma^{s_a-1} + (1 + \gamma +... + \gamma^{t-1})\gamma^{s_a}\hat{p}_{k, t}^\gamma}{1 + \gamma +... + \gamma^{t + s_a-1}},
\end{align*}
where $\hat{p}_{k, t}^\gamma = \frac{\mathbbm{1}_{(a_{t} = k|p_{k,t})}\gamma^{0} + ... + \mathbbm{1}_{(a_{1} = k|p_{k,1})}\gamma^{t-1}}{1 + \gamma +... + \gamma^{t -1}}$.
And then we can compute the expected value of $\hat{p}_{k, t+s_a}^\gamma$, namely,
\begin{align*}
\Esymb[\hat{p}_{k, t+s_a}^\gamma| \hat{p}_{k, t}^\gamma, \vp(m+1) = \vp_e] & = \frac{p_k\gamma^0 + p_k\gamma^1 + ... + p_k\gamma^{s_a-1} + (1 + \gamma +... + \gamma^{t-1})\gamma^{s_a}\hat{p}_{k, t}^\gamma}{1 + \gamma +... + \gamma^{t + s_a-1}} \\
% & = \frac{p_k \frac{1-\gamma^{s_a}}{1-\gamma}+  \frac{1-\gamma^{t}}{1-\gamma}\gamma^{s_a}\hat{p}_{k, t}^\gamma}{\frac{1-\gamma^{t+s_a}}{1-\gamma}} \\
& = \frac{p_k(1-\gamma^{s_a}) + \hat{p}_{k,t}^\gamma\gamma^{s_a}(1-\gamma^{t})}{1-\gamma^{t+s_a}} .
% & = \frac{p_k + \gamma^{s_a}(\hat{p}_{k,t}^\gamma(1-\gamma^t) - p_k)}{1-\gamma^{t+s_a}}
\end{align*}
Furthermore, we have
\begin{align*}
\big|\Esymb[\hat{p}_{k, t+s_a}^\gamma| \hat{p}_{k, t}^\gamma, \vp(m+1)  = \vp_e] - p_k\big| & =  \bigg|\frac{p_k(1-\gamma^{s_a}) + \hat{p}_{k,t}^\gamma\gamma^{s_a}(1-\gamma^{t})}{1-\gamma^{t+s_a}} - p_k \bigg| \\
% & = \bigg|\frac{p_k(1-\gamma^{s_a}) + \hat{p}_{k,t}^\gamma\gamma^{s_a}(1-\gamma^t) - p_k(1-\gamma^{t+s_a})}{1-\gamma^{t+s_a}}\bigg| \\
% & = \bigg|\frac{p_k(\gamma^{t+s_a} - \gamma^{s_a}) + \hat{p}_{k,t}^\gamma\gamma^{s_a}(1-\gamma^t)}{1-\gamma^{t+s_a}}\bigg| \\
% & = \bigg|\frac{\gamma^{s_a}(1-\gamma^t)(\hat{p}_{k,t}^\gamma - p_k)}{1-\gamma^{t+s_a}}\bigg| \\
& \leq \frac{\gamma^{s_a}(1-\gamma^{t})}{1-\gamma^{t+s_a}} < \gamma^{s_a}.
\end{align*}

Recall that $U(\vp) = \sum_{p_k \in \vp} p_k\mu_k(p_k)$.
In the estimation stage, we approximate all the realized rewards as the rewards generated by the meta arm $\vp_e$.
\ignore{
	Firstly, according to above weighted sum Hoeffding's inequality (\ref{hoeffding: weights}),  we have:
	\begin{align}
	\Psymb\bigg(\big|U(\vp_e) - \overbar{U}_{mL}^\est(\vp_e) \big| \geq \delta \bigg) \leq 2\exp\bigg(-\frac{2\delta^2}{\sum_{p_k\in\vp_e} \frac{1}{n^\est_{mL}(p_k)}}\bigg) \leq 2\exp\bigg(-\frac{2\delta^2n_{mL}^\est(\underline{p}_k)}{K} \bigg)
	\end{align}
	where $\underline{p}_k = \argmin_{p_k\in\vp} n_{mL}^\est(p_k)$ and $n_{mL}^\est(p_k) = (L-s_a)\sum_{i = 1}^{m+1} \mathbbm{1}(p_k \in \vp(i))$.

	Thus, let $\delta = \sqrt{\frac{K\ln \big(L\rho_em \big)}{{n_{mL}^\est(\underline{p}_k)}}}$, then with probability at least $1-\frac{2}{(L\rho_em )^2}$,
	\begin{align}
	\bigg|U(\vp_e) - \overbar{U}_{mL}^\est(\vp_e) \bigg| \leq \sqrt{\frac{K\ln \big(L\rho_em\big)}{n_{mL}^\est(\underline{p}_k)}}
	\end{align}
}
However, note that we acutally cannot compute the value of $\overbar{U}_{mL}^\est(\vp_e)$, instead, we use $\overbar{U}_{mL}^\est(\hat{\vp}_{e, t+s_a}^\gamma)$ of each phase as an approximation of $\overbar{U}_{mL}^\est(\vp_e)$, i.e., we approximate all $\hat{\vp}_{e, t+s}^\gamma, \forall s \in (s_a, L]$ as $\hat{\vp}_{e, t+s_a}^\gamma$ given $\vp(m+1) = \vp_e$.
Recall that for any $s\in (s_a, L]$, we have:
\begin{align*}
\big|\Esymb[\hat{p}_{k, t+s}^\gamma| \hat{p}_{k, t}^\gamma, \vp(m+1)  = \vp_e] - p_k\big| & = \bigg|\frac{\gamma^{s}(1-\gamma^t)(\hat{p}_{k,t}^\gamma - p_k)}{1-\gamma^{t+s}}\bigg| \\
& \leq \frac{\gamma^{s}(1-\gamma^{t})}{1-\gamma^{t+s}} < \frac{\gamma^{s_a}(1-\gamma^{t})}{1-\gamma^{t+s_a}} < \gamma^{s_a}.
\end{align*}
Thus, the approximation error on the empricial estimation can be computed as follows:
\begin{align*}
\Esymb \big[\big|\overbar{U}_{mL}^\est(\hat{\vp}_{e, t+s_a}^\gamma) -  \overbar{U}_{mL}^\est(\vp_e)\big| \big] & = \Esymb \bigg[\bigg|\sum_{p_k^\gamma \in \hat{\vp}_{e, t+s_a}^\gamma} p_k^\gamma\bar{r}^\est_{t+s_a}(p_k^\gamma) - \sum_{p_k \in \vp_e} p_k\bar{r}^\est_{t+s_a}(p_k)\bigg|\bigg]\\
& = \bigg|\sum \bigg((p_k^\gamma-p_k) \Esymb\big[\bar{r}^\est_{t+s_a}(p_k^\gamma) - \bar{r}^\est_{t+s_a}(p_k)\big]\bigg) \bigg|\\
& = \bigg|\sum \bigg((p_k^\gamma-p_k) \big(\mu_k(p_k^\gamma) - \mu_k(p_k)\big)\bigg) \bigg|\\
& = \sum \gamma^{s_a}\cdot L_k\gamma^{s_a} \leq K\gamma^{2s_a}L^*,
\end{align*}
where the third equation is by law of total expectation and recall that $L^* = \max_{k\in[K]} L_k$.
\end{proof}

\subsection{Proof of Lemma \ref{lemma:high_prob_error_neq_1}}
\begin{proof}
By decomposing $\big|U(\vp_e) - \overbar{U}_{mL}^\est(\hat{\vp}_{e, t+s_a}^\gamma)\big|$ and applying the Hoeffding's Inequality on Weighted Sums, we'll have
\begin{align*}
& \Psymb\bigg(\big|U(\vp_e) - \overbar{U}_{mL}^\est(\hat{\vp}_{e, t+s_a}^\gamma)\big| \geq \delta\bigg) \\
\leq & \Psymb\bigg(\big|U(\vp_e) - \overbar{U}_{mL}^\est(\vp_e)  \big|  + \big|\overbar{U}_{mL}^\est(\vp_e) - \overbar{U}_{mL}^\est(\hat{\vp}_{e, t+s_a}^\gamma)  \big|  \geq \delta\bigg) \\
= & \Psymb\bigg(\big|U(\vp_e) - \overbar{U}_{mL}^\est(\vp_e)  \big|  + \big|\overbar{U}_{mL}^\est(\hat{\vp}_{e, t+s_a}^\gamma) - \Esymb[\overbar{U}_{mL}^\est(\hat{\vp}_{e, t+s_a}^\gamma) ]\\
&  \quad \quad - (\overbar{U}_{mL}^\est(\vp_e) - \Esymb[\overbar{U}_{mL}^\est(\vp_e)] ) + \Esymb[\overbar{U}_{mL}^\est(\vp_e)] - \Esymb[\overbar{U}_{mL}^\est(\hat{\vp}_{e, t+s_a}^\gamma) ] \big|  \geq \delta\bigg)\\
\leq  & \Psymb\bigg(2\big|U(\vp_e) - \overbar{U}_{mL}^\est(\vp_e)  \big|  + \big|\overbar{U}_{mL}^\est(\hat{\vp}_{e, t+s_a}^\gamma) - \Esymb[\overbar{U}_{mL}^\est(\hat{\vp}_{e, t+s_a}^\gamma)\big| \geq \delta - \err\bigg)\\
\leq &  3\Psymb\bigg(|U(\vp_e) - \overbar{U}_{mL}^\est(\vp_e)  \big|  \geq \frac{\delta - \err}{3}\bigg)\\
\leq & 6\exp\bigg(-\frac{\underline{n}^\est_{mL}(p_k)(\delta - \err)^2}{9K} \bigg).
\end{align*}
\end{proof}

\subsection{Proof of Lemma \ref{lemma:key_lemma_neq_1}} \label{proof_of_lemma:key_lemma_neq_1}
\begin{proof}
By the definition of the constructed $\UCB$, we'll have
\begin{align*}
\UCB_{mL}(\vp) & =  \overbar{U}_{mL}^\est(\hat{\vp}_{ t+s_a}^\gamma) + \err + 3\sqrt{\frac{K\ln \big(L\rho_em\big)}{n_{mL}^\est(\underline{p}_k)}} \\
& \leq \overbar{U}_{mL}^\est(\hat{\vp}_{ t+s_a}^\gamma) + \frac{\Delta_{\vp}}{2} \\
& < \big(U(\vp) + \frac{\Delta_{\vp}}{2}\big) + \frac{\Delta_{\vp}}{2}  \\
& = U(\vp^*)  < \UCB_{mL}(\vp^*),
\end{align*}
where the first inequality is due to  $n_{mL}^\est(\underline{p}_k) \geq \frac{9K\ln \big(L\rho_em\big)}{\big(\frac{\Delta_{\vp}}{2} - \err\big)^2}$,
and the probability of third or fifth inequality not holding is at most $\frac{12}{\big(L\rho_em\big)^2}$.
\end{proof}

\subsection{Proof of Lemma \ref{lemma: sufficient_sample_reduction}}\label{proof_of_lemma: sufficient_sample_reduction}
\begin{proof} 
For each suboptimal arm $\vp \neq \vp^*$, and suppose there exists $\underline{p}_{k,j_k} \notin \vp^*$ such that $\underline{p}_{k,j_k} = \argmin_{p_{k,j_k} \in \vp} n^\est_t(p_{k,j_k})$, then
\begin{align*}
\Esymb[n^\est_t(\underline{p}_{k,j_k})] & = (L-s_a)\Esymb \bigg[\sum_{i = 1}^{m} \mathbbm{1}\bigg(\vp(i) = \vp, \vp\in \cS(\underline{p}_{k,j_k})\bigg)\bigg] \\
& =(L-s_a) \Esymb \bigg[\sum_{i = 1}^{m} \mathbbm{1}\bigg(\vp(i) = \vp, \vp\in \cS(\underline{p}_{k,j_k}); n_{iL}^\est(\underline{p}_{k,j_k}) < \frac{9K\ln \big(i(L-s_a)\big)}{\big(\frac{\Delta_{\vp}}{2} - \err\big)^2} \bigg)\bigg] + \\
& \quad  (L-s_a)\Esymb \bigg[\sum_{i = 1}^{m} \mathbbm{1}\bigg(\vp(i) = \vp, \vp\in \cS(\underline{p}_{k,j_k}); n_{iL}^\est(\underline{p}_{k,j_k}) \geq \frac{9K\ln \big(i(L-s_a)\big)}{\big(\frac{\Delta_{\vp}}{2} - \err\big)^2}\bigg)\bigg] \\
& \leq \frac{9K\ln \big(t^\est_{m}\big)}{\big(\frac{\Delta_{\vp}}{2} - \err\big)^2} +  (L-s_a)\Esymb \bigg[\sum_{i = 1}^{m} \mathbbm{1}\bigg(\vp(i) = \vp, \vp\in \cS(\underline{p}_{k,j_k}); n_{iL}^\est(\underline{p}_{k,j_k}) \geq \frac{9K\ln \big(i(L-s_a)\big)}{\big(\frac{\Delta_{\vp}}{2} - \err\big)^2} \bigg)\bigg] \\
& = \frac{9K\ln \big(t^\est_{m}\big)}{\big(\frac{\Delta_{\vp}}{2} - \err\big)^2} +  (L-s_a)\sum_{i = 1}^{m}\Psymb \bigg(\vp(i) = \vp, \vp\in \cS(\underline{p}_{k,j_k}); n_{iL}^\est(\underline{p}_{k,j_k}) \geq \frac{9K\ln \big(i(L-s_a)\big)}{\big(\frac{\Delta_{\vp}}{2} - \err\big)^2}\bigg) \\
& = \frac{9K\ln \big(t^\est_{m}\big)}{\big(\frac{\Delta_{\vp}}{2} - \err\big)^2} +  (L-s_a) \sum_{i = 1}^{m} \Psymb\bigg(\vp(i) = \vp, \vp\in \cS(\underline{p}_{k,j_k})\bigg| n_{iL}^\est(\underline{p}_{k,j_k}) \geq \frac{9K\ln \big(i(L-s_a)\big)}{\big(\frac{\Delta_{\vp}}{2} - \err\big)^2} \bigg) \cdot\\
& \qquad \qquad \qquad \qquad \qquad \qquad \qquad \qquad \qquad \Psymb \bigg(n_{iL}^\est(\underline{p}_{k,j_k}) \geq \frac{9K\ln \big(i(L-s_a)\big)}{\big(\frac{\Delta_{\vp}}{2} - \err\big)^2}\bigg)\\
& \leq  \frac{9K\ln \big(t^\est_{m}\big)}{\big(\frac{\Delta_{\vp}}{2} - \err\big)^2} + (L-s_a)\sum_{i=1}^{m} \frac{12}{\big(i(L-s_a)\big)^2}\\
% & = (L-s_a)\frac{9K\ln \big(t^\est_{m}\big)}{\big(\frac{\Delta_{\vp}}{2} - \err\big)^2} + 12(L-s_a)\bigg(\frac{1}{(L-s_a)^2}+ \frac{1}{(2(L-s_a))^2} +... +\frac{1}{(m(L-s_a))^2}\bigg) \\
% & = \frac{9K\ln \big(t^\est_{m}\big)}{\big(\frac{\Delta_{\vp}}{2} - \err\big)^2} + \frac{12}{L-s_a}\bigg(\frac{1}{1}+ \frac{1}{2^2} +... +\frac{1}{m^2}\bigg)\\
& \leq \frac{9K\ln \big(t^\est_{m}\big)}{\big(\frac{\Delta_{\vp}}{2} - \err\big)^2} + \frac{2\pi^2}{L-s_a}.
\end{align*}
For the first inequality, suppoese for contradiction that the indicator $\mathbbm{1}\big(\vp(t) = \vp, \vp\in \cS(\underline{p}_{k,j_k}); n_{mL}^\est(\underline{p}_{k,j_k}) < L\big)$ takes value of 1 at more than $L-1$ time steps, where $L = \frac{9K\ln \big(m(L-s_a)\big)}{\big(\frac{\Delta_{\vp}}{2} - \err\big)^2}$. 
Let $\tau$ be the time step at which this indicator is 1 for the $(L-1)-th$ time.
Then the number of pulls of all meta arms in $\cS(\underline{p}_{k,j_k})$ is at least $L$ times until time $\tau$ (including the initial pull), and for all $t > \tau$, $n_t(\underline{p}_{k,j_k}) \geq L$ which implies $n_{mL}^\est(\underline{p}_{k,j_k}) \geq \frac{9K\ln \big(m(L-s_a)\big)}{\big(\frac{\Delta_{\vp}}{2} - \err\big)^2}$.
Thus, the indicator cannot be 1 for any $t\geq \tau$, contradicting the assumption that the indicator takes value of 1 more than $L$ times.
This bounds $1 + \Esymb \big[\sum_{t = n}^T \mathbbm{1}\big(\vp(t) = \vp, \vp\in \cS(\underline{p}_{k,j_k}); n_{mL}^\est(\underline{p}_{k,j_k}) < L\big)\big]$ by $L$.
\end{proof}

\subsection{Proof of Theorem \ref{theorem: key_theorem_neq_1}} \label{proof_of_theorem: key_theorem_neq_1}
\begin{proof}
The total regret is defined as follows:
\begin{align*}
\Esymb[R(t)] & = \sum_{\vp\neq \vp^*}N_t(\vp)\Delta_{\vp}\\
& = \sum_{p_{k,j_k}\notin \vp^*}\sum_{l\in[L^{p_{k,j_k}}]}N_t(\vp_l(p_{k,j_k}))\Delta_l^{p_{k,j_k}},
\end{align*}
where $N_t(\vp) = L \sum_{i = 1}^{\left \lfloor t/L \right \rfloor} \mathbbm{1}\big(\vp(i) = \vp\big)$.
Suppose we choose $s_a$ to satisfy that $\min_{\vp}\Delta_{\vp} > 2\err$.

% Define $l_t^\gamma(\Delta) \overset{\Delta}{=}  \frac{9KL\ln \big(t(L-s_a)/L\big)}{\big(\frac{\Delta}{2} - \err\big)^2} + \frac{2L\pi^2}{(L-s_a)^2}$.
Define $l_t^\gamma(\Delta) \overset{\Delta}{=}  \frac{9K\ln \big(t\rho_e\big)}{\rho_e\big(\frac{\Delta_{\vp}}{2} - \err\big)^2} + \frac{2\pi^2}{L\rho_e^2}$.
Follow the same logic from (\ref{ineq: relax_badness_1}) to (\ref{logics_end: relax gap}), we have:
\begin{align*}
\sum_{l\in[L^{p_{k,j_k}}]}N_t(\vp_l(p_{k,j_k}))\Delta_l^{p_{k,j_k}} 
\leq & \quad \sum_{j=1}^{L^{p_{k,j_k}}} \big(l_t^\gamma(\Delta_j^{p_{k,j_k}}) - l_t^\gamma(\Delta_{j-1}^{p_{k,j_k}})\big) \Delta_j^{p_{k,j_k}} \\
= 	 & \quad l_t^\gamma(\Delta_\text{min}^{p_{k,j_k}})\Delta_\text{min}^{p_{k,j_k}} + \sum_{j \in [L^{p_{k,j_k}} - 1]}l_t^\gamma(\Delta_j^{p_{k,j_k}})\cdot(\Delta_j^{p_{k,j_k}} - \Delta_{j+1}^{p_{k,j_k}}) \\
\leq & \quad l_t^\gamma(\Delta_\text{min}^{p_{k,j_k}})\Delta_\text{min}^{p_{k,j_k}} +  \quad \int_{\Delta_\text{min}^{p_{k,j_k}}}^{\Delta_\text{max}^{p_{k,j_k}}}l_t^\gamma(x)dx \\
% =    & \quad \frac{9\Delta_\text{min}^{p_{k,j_k}}KL\ln \big(t(L-s_a)/L\big)}{\big(\frac{\Delta_\text{min}^{p_{k,j_k}}}{2} - \err\big)^2} + \frac{2\Delta_\text{min}^{p_{k,j_k}}L\pi^2}{(L-s_a)^2} +  \int_{\Delta_\text{min}^{p_{k,j_k}}}^{\Delta_\text{max}^{p_{k,j_k}}} \bigg(\frac{9KL\ln \big(t(L-s_a)/L\big)}{\big(\frac{x}{2} - \err\big)^2} + \frac{2L\pi^2}{(L-s_a)^2}\bigg)dx\\
% =    & \quad \frac{9\Delta_\text{min}^{p_{k,j_k}}KL\ln \big(t(L-s_a)/L\big)}{\big(\frac{\Delta_\text{min}^{p_{k,j_k}}}{2} - \err\big)^2} + \frac{2\Delta_\text{max}^{p_{k,j_k}}L\pi^2}{(L-s_a)^2} + \quad 9KL\ln \big(t(L-s_a)/L\big) \bigg(\frac{2}{\frac{\Delta_\text{min}^{p_{k,j_k}}}{2} - \err} - \frac{2}{\frac{\Delta_\text{max}^{p_{k,j_k}}}{2} - \err}\bigg)\\
% \leq & \quad 9KL\ln \bigg(\frac{t(L-s_a)}{L}\bigg) \bigg(\frac{\Delta_\text{min}^{p_{k,j_k}}}{\big(\frac{\Delta_\text{min}^{p_{k,j_k}}}{2} - \err\big)^2} + \frac{2}{\frac{\Delta_\text{min}^{p_{k,j_k}}}{2} - \err} - \frac{4}{1 - 2\err}\bigg) +  \frac{2L\pi^2}{(L-s_a)^2} 
=    & \quad \frac{9\Delta_\text{min}^{p_{k,j_k}}K\ln \big(t\rho_e\big)}{\rho_e\big(\frac{\Delta_\text{min}^{p_{k,j_k}}}{2} - \err\big)^2} + \frac{2\Delta_\text{min}^{p_{k,j_k}}\pi^2}{L\rho_e^2} +  \int_{\Delta_\text{min}^{p_{k,j_k}}}^{\Delta_\text{max}^{p_{k,j_k}}} \bigg(\frac{9K\ln \big(t\rho_e\big)}{\rho_e\big(\frac{x}{2} - \err\big)^2} + \frac{2\pi^2}{L\rho_e^2}\bigg)dx\\
=    & \quad \frac{9\Delta_\text{min}^{p_{k,j_k}}K\ln \big(t\rho_e\big)}{\rho_e\big(\frac{\Delta_\text{min}^{p_{k,j_k}}}{2} - \err\big)^2} + \frac{2\Delta_\text{max}^{p_{k,j_k}}\pi^2}{L\rho_e^2}  + \frac{9K\ln \big(t\rho_e\big)}{\rho_e} \bigg(\frac{2}{\frac{\Delta_\text{min}^{p_{k,j_k}}}{2} - \err} - \frac{2}{\frac{\Delta_\text{max}^{p_{k,j_k}}}{2} - \err}\bigg)\\
\leq & \quad  \frac{9K\ln \big(t\rho_e\big)}{\rho_e} \bigg(\frac{\Delta_\text{min}^{p_{k,j_k}}}{\big(\frac{\Delta_\text{min}^{p_{k,j_k}}}{2} - \err\big)^2} + \frac{2}{\frac{\Delta_\text{min}^{p_{k,j_k}}}{2} - \err} - \frac{4}{1 - 2\err}\bigg) +  \frac{2\pi^2}{L\rho_e^2}.
\end{align*}
% \wt{didn't have an intuitive idea where we should optimize $L$, this may be caused by above relaxation issue.}
Thus, the total regret can be bounded as follows:
\begin{align*}
% \Esymb[R(t)] \leq \sum_{p_{k,j_k}\notin \vp^*}\bigg( 9KL\ln \bigg(\frac{t(L-s_a)}{L}\bigg) \bigg(\frac{\Delta_\text{min}^{p_{k,j_k}}}{\big(\frac{\Delta_\text{min}^{p_{k,j_k}}}{2} - \err\big)^2} + \frac{2}{\frac{\Delta_\text{min}^{p_{k,j_k}}}{2} - \err} - \frac{4}{1 - 2\err}\bigg) +  \frac{2L\pi^2}{(L-s_a)^2} \bigg)
\Esymb[R(t)] \leq \sum_{p_{k,j_k}\notin \vp^*}\bigg( \frac{9K\ln \big(t\rho_e\big)}{\rho_e} \bigg(\frac{\Delta_\text{min}^{p_{k,j_k}}}{\big(\frac{\Delta_\text{min}^{p_{k,j_k}}}{2} - \err\big)^2} + \frac{2}{\frac{\Delta_\text{min}^{p_{k,j_k}}}{2} - \err} - \frac{4}{1 - 2\err}\bigg) +  \frac{2\pi^2}{L\rho_e^2}\bigg).
\end{align*}
Below we provide an instance-independent regret.
Define $\Delta^* = 2\sqrt{\frac{K^2\ln (t\rho_e)}{\epsilon t} } + 2\err$.
Considering following two cases:
\squishlist
	\item Group 1 contains the super sets which satisfy $\Delta_\text{min}^{p_{k,j_k}} \geq \Delta^*$;
	\item Group 2 contains the super sets which satisfy  $\Delta_\text{min}^{p_{k,j_k}} < \Delta^*$.
\squishend
For the case 1, the maximum total regret incurred due to pulling the suboptimal meta arms is bounded by:
\begin{align*}
& \sum_{\vp \in \{\cup_{\cS: \cS\in \text{Group 1}} \cS\} } N_t(\vp)\Delta_{\vp} \\
% \leq & \sum_{p_{k,j_k} \in \text{Group 1}} \bigg(\frac{9K\ln \big(t\rho_e\big)}{\rho_e} \bigg(\frac{\Delta_\text{min}^{p_{k,j_k}}}{\big(\frac{\Delta_\text{min}^{p_{k,j_k}}}{2} - \err\big)^2} + \frac{2}{\frac{\Delta_\text{min}^{p_{k,j_k}}}{2} - \err} - \frac{4}{1 - 2\err}\bigg) +  \frac{2\pi^2}{L\rho_e^2}\bigg)  \\
\leq & \sum_{p_{k,j_k} \in \text{Group 1}} \bigg( \frac{9K\ln \big(t\rho_e\big)}{\rho_e} \bigg(\frac{2\sqrt{\frac{K^2\ln (t\rho_e)}{\epsilon t} } + 2\err}{\frac{K^2\ln (t\rho_e)}{\epsilon t}} + 2\sqrt{\frac{\epsilon t}{K^2\ln (t\rho_e)}} - \frac{4}{1 - 2\err} \bigg) +  \frac{2\pi^2}{L\rho_e^2}\bigg) \\
 = & \sum_{p_{k,j_k} \in \text{Group 1}} \bigg(18\bigg(\frac{2\sqrt{\epsilon t\ln(t\rho_e)}} {\rho_e} + \frac{ \epsilon t \err }{K\rho_e} - \frac{2K\ln(t\rho_e)}{\rho_e(1-2\err)} \bigg) +  \frac{2\pi^2}{L\rho_e^2}\bigg) \\
% \leq & \frac{K}{\epsilon} \bigg(18\bigg(\frac{2\sqrt{K\epsilon t\ln(t\rho_e)}} {\rho_e} + \frac{ \epsilon t \err }{\rho_e} - \frac{2K\ln(t\rho_e)}{\rho_e(1-2\err)} \bigg) +  \frac{2\pi^2}{L\rho_e^2}\bigg) \\
\leq & 18\bigg(\frac{2K\sqrt{\frac{t\ln(t\rho_e)}{\epsilon}}} {\rho_e} + \frac{ t \err }{\rho_e} - \frac{2K^2\ln(t\rho_e)}{\rho_e\epsilon(1-2\err)} \bigg) + \frac{2K\pi^2}{L\epsilon\rho_e^2}.
\end{align*}
For the case 2, the maximum total regret incurred due to pulling the suboptimal meta arms is bounded by:
\begin{align*}
\sum_{\vp \in \{\cup_{\cS: \cS\in \text{Group 2}} \cS\} } N_t(\vp)\Delta_{\vp} & \leq \Delta^* \sum_{\vp \in \{\cup_{\cS: \cS\in \text{Group 2}} \cS\} } N_t(\vp) \leq t\Delta^*\\
& =  2K\sqrt{\frac{t\ln (t \rho_e)}{\epsilon}} + 2t\err.
\end{align*}
So the total regret incurred by above two cases are:
\begin{align*}
\Esymb_{\cA}[R(t)] \leq \frac{36K + 2\rho_e}{\rho_e}\sqrt{\frac{t\ln (t \rho_e)}{\epsilon}} + \frac{18 + 2\rho_e}{\rho_e} t\err - \frac{36K^2\ln(t\rho_e)}{\rho_e\epsilon(1-2\err)}+ \frac{2K\pi^2}{L\epsilon\rho_e^2}.
\end{align*}
Combine with the discretization error, we have:
\begin{align} 
\Esymb[R(t)] & = \Esymb_{\cA}[R(t)]  + \DE_\epsilon\\
& = \frac{36K + 2\rho_e}{\rho_e}\sqrt{\frac{t\ln (t \rho_e)}{\epsilon}} + \frac{18 + 2\rho_e}{\rho_e} t\err - \frac{36K^2\ln(t\rho_e)}{\rho_e\epsilon(1-2\err)}+ \frac{2K\pi^2}{L\epsilon\rho_e^2} + Ct(K-1)\epsilon \\
& <  \frac{36K + 2\rho_e}{\rho_e}\bigg(\sqrt{\frac{t\ln (t \rho_e)}{\epsilon}} + t\err\bigg) - \frac{36K^2\ln(t\rho_e)}{\rho_e\epsilon(1-2\err)}+ \frac{2K\pi^2}{L\epsilon\rho_e^2} + CtK\epsilon.  \label{eq: regret_gamma}
\end{align}
Optimizing (\ref{eq: regret_gamma}) w.r.t $\epsilon$, i.e., we solve optimal $\epsilon$ by letting $CtK\epsilon =  \frac{36K + 2\rho_e}{\rho_e}\sqrt{\frac{t\ln (t \rho_e)}{\epsilon}}$, i.e.,
\begin{align} \label{eq: optimal_epsilon}
\epsilon^* = \bigg(\frac{(36K + 2\rho_e)^2 \ln (t\rho_e)}{C^2K^2t\rho_e^2}\bigg)^{1/3} = \Theta\bigg(t^{-1/3}\big(\ln(t\rho_e)\big)^{1/3}\bigg).
\end{align}
Plug back and then optimize (\ref{eq: regret_gamma}) w.r.t $\err = KL^*\gamma^{2s_a}$, i.e., we solve optimal $s_a^*$ by letting $t\err =  \sqrt{\frac{t\ln (t \rho_e)}{\epsilon}}$, i.e.,
\begin{align} \label{eq: optimal_s_a}
s_a^* = \frac{\ln \bigg(\frac{1}{KL^*}\sqrt{\frac{\ln (t\rho_e)}{t\epsilon}} \bigg)}{2\ln \gamma} = \Theta\bigg(\frac{\ln \bigg(\frac{\ln(t\rho_e)}{tK^3}\bigg)^{1/3}}{\ln \gamma}\bigg),
\end{align}
where the last equality is by plugging in optimal $\epsilon^*$ computed from (\ref{eq: optimal_epsilon}).

So given any constant ratio $\rho_e$, and divide $T$ into consecutive phases with a length of $L = \frac{s_a^*}{1-\rho_e}$ and ensure the length of approaching stage (i.e., $s_a^*$) of each phase satsfies (\ref{eq: optimal_s_a}),
we then have following regret bound:
\begin{align*}
\Esymb[R(t)] & = \frac{3(36K+2\rho_e)}{\rho_e} \sqrt{\frac{t\ln(t\rho_e)}{\big(\frac{(36K + 2\rho_e)^2 \ln (t\rho_e)}{C^2K^2t\rho_e^2}\big)^{1/3}}} -  \frac{36K^2\ln(t\rho_e)}{\rho_e\epsilon(1-2\err)}+ \frac{2K\pi^2}{L\epsilon\rho_e^2} \\
& < \frac{3(36K+2\rho_e)}{\rho_e} \sqrt{\frac{K^{2/3}t^{4/3}(\ln(t\rho_e))^{2/3}\rho_e^{2/3}C^{2/3}}{(36K+2\rho_e)^{2/3}}} + \frac{2K\pi^2}{L\rho_e^2}\bigg(\frac{C^2Kt\rho_e^2}{(36K + 2\rho_e)^2 \ln (t\rho_e)}\bigg)^{1/3} \\
% & < \frac{3\cdot38K}{\rho_e} \frac{K^{2/3}t^{2/3}(\ln(t\rho_e))^{1/3}\rho_e^{1/3}C^{1/3}}{(36K)^{1/3}} + \frac{2K\pi^2}{}\\
& = \cO\bigg(\frac{K t^{2/3}\big(\ln (t\rho_e)\big)^{1/3}}{(\rho_e)^{2/3}} \bigg) + \cO\bigg(\frac{K^{2/3}t^{1/3}}{\rho_e^{4/3}(\ln(t\rho_e))^{1/3}}\bigg) \label{eq: optimizing_rho_e}\\
& \leq \cO\bigg(\frac{K t^{2/3}\big(\ln (t\rho_e)\big)^{1/3}} {(\rho_e)^{2/3}} \bigg).
\end{align*}
\end{proof}

% --------------------------------------------------------------
\section{Missing Proofs for the Lower Bound in Section \ref{sec: lower_bound}} \label{appendix: proofs_lower_bound}

\subsection{Proof of Lemma \ref{lemma: regret_mapping}} \label{proof_regret_mapping}
% \wt{needs more work to make the notations consistent.}

\subsection{Proof of Step 2} \label{proof_lower_bound_step_2}

\subsection{Proof of Step 3} \label{proof_lower_bound_step_3}
